# Supplementary material for: Topological Solitons versus Non-Solitonic Phase Defects in Quasi-One-Dimensional Charge Density Wave
Source: arXiv:1211.5440 source file (2012-11-23)
Supplement: Supplementary file 1 [file soliton_supporting_info_small.pdf]

# Supplemental Material for: Topological Solitons versus Non-Solitonic Phase Defects in Quasi-One-Dimensional Charge Density Wave

Tae-Hwan Kim* and Han Woong Yeom†

*Center for Low Dimensional Electronic Symmetry and Department of Physics, Pohang University of Science and Technology, Pohang 790-784, Korea*

* taehwan@postech.ac.kr

† yeom@postech.ac.kr

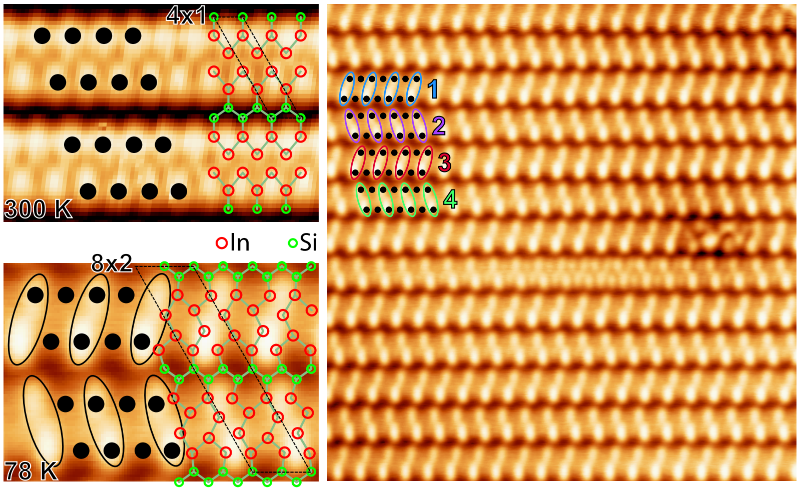


FIG. S1. Left panel shows atomic STM images obtained above (300 K, top) and below the CDW transition temperature (78 K, bottom), respectively. At 300 K, an In wire of Si(111)4×1-In has two In atomic chains (black dots in a simplified model of Fig. 1 and red circles in a realistic atomic model) and is separated by Si chains (green circles) [1, 2]. Upon cooling, each In atomic chain undergoes a periodicity-doubling distortion along a wire, resulting in a four-fold degeneracy of a 4×2 CDW state (indicated by tilted ovals in left bottom panel). As shown in the inset of Fig. 1(a), four energetically equivalent ground states of $4 \times 2$ CDW wires are highlighted by colors and numbers in the right panel. In addition, interwire coupling forces CDW wires to have opposite tilting angles alternatively perpendicular to the wire, leading to 8×2 ordering (left bottom and right panels). If a 4×2 CDW wire is type 1 or 3 (blue or red ovals), next neighboring wires should be either type 2 or 4 (violet or green ovals), and vice versa.


[1] S. J. Park *et al.*, Phys. Rev. Lett. **93**, 106402 (2004).

[2] C. González *et al.*, Phys. Rev. Lett. **102**, 115501 (2009).

[3] I. Tüttő and A. Zawadowski, Phys. Rev. B **32**, 2449 (1985).

[4] S. Brazovskii, C. Brun, Z.-Z. Wang, and P. Monceau, Phys. Rev. Lett. **108**, 096801 (2012).

[5] H. Zhang *et al.*, Phys. Rev. Lett. **106**, 026801 (2011).

[6] T. Uetake *et al.*, Phys. Rev. B **86**, 035325 (2012).

[7] J. R. Ahn *et al.*, Phys. Rev. Lett. **93**, 106401 (2004).

[8] Yu. I. Latyshev *et al.*, Phys. Rev. Lett. **95**, 266402 (2005).

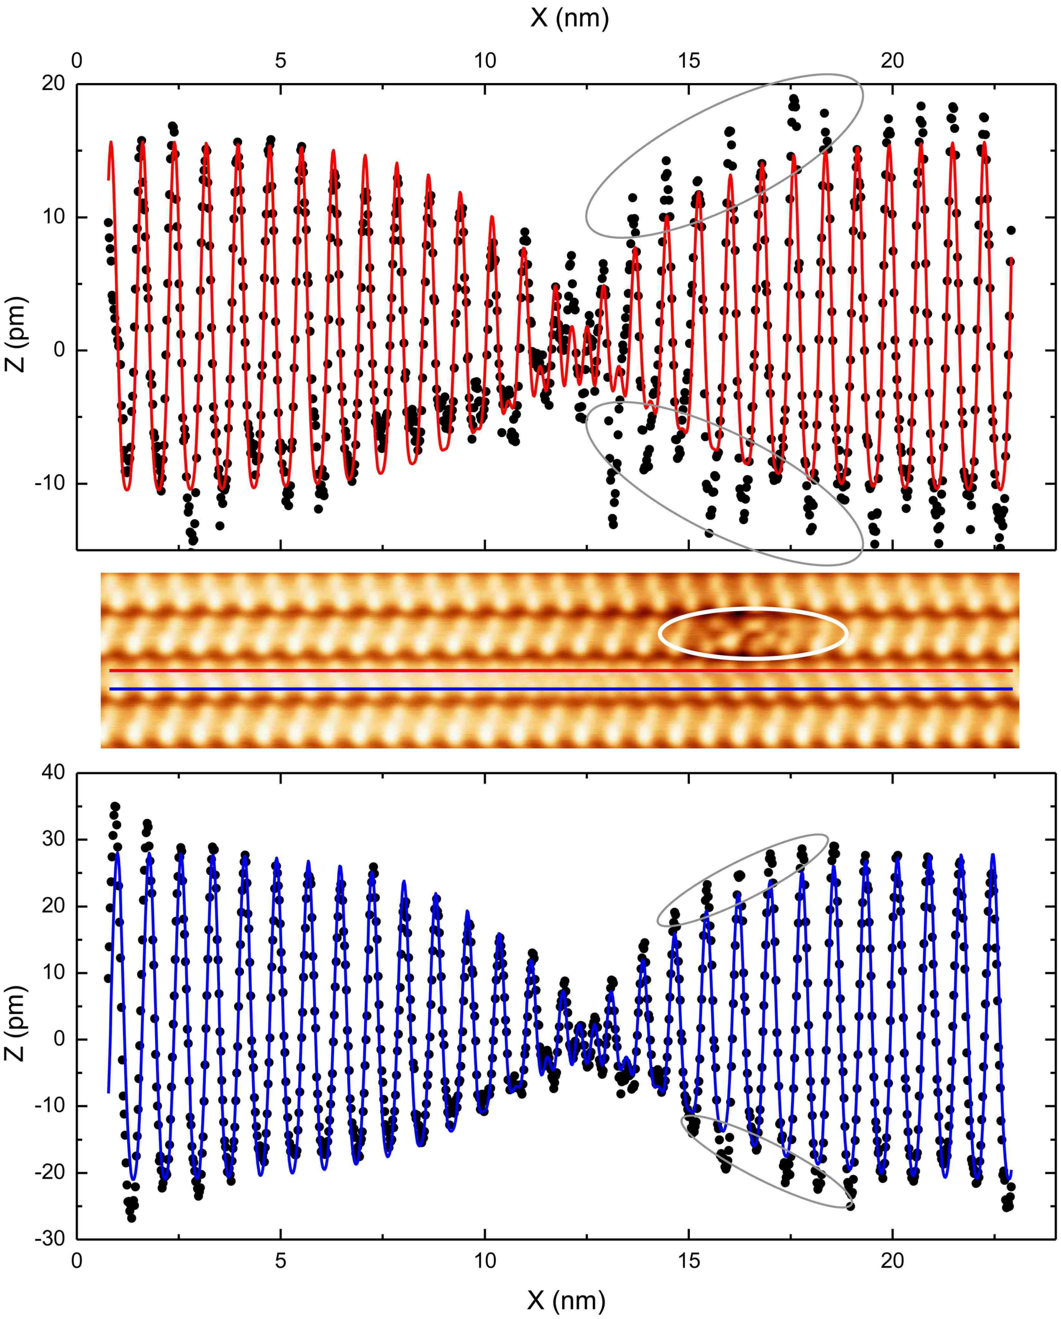


FIG. S2. Two STM line profiles (dots) from a long phase slip defect in Fig. 1(c) along two In atomic chains, closer (red line) to and farther (blue line) from the short phase slip defect. Red and blue solid lines represent the best fits of the corresponding STM profiles (marked by the same color lines in the STM image). The deviations from the soliton profiles are clearly observed near the neighboring defect as highlighted by the ovals. In addition, the deformation of a soliton appears more significantly on the In atomic chain closer to the short phase slip defect (red line). This clearly indicates that the deformation of CDW is induced by the neighboring defect.

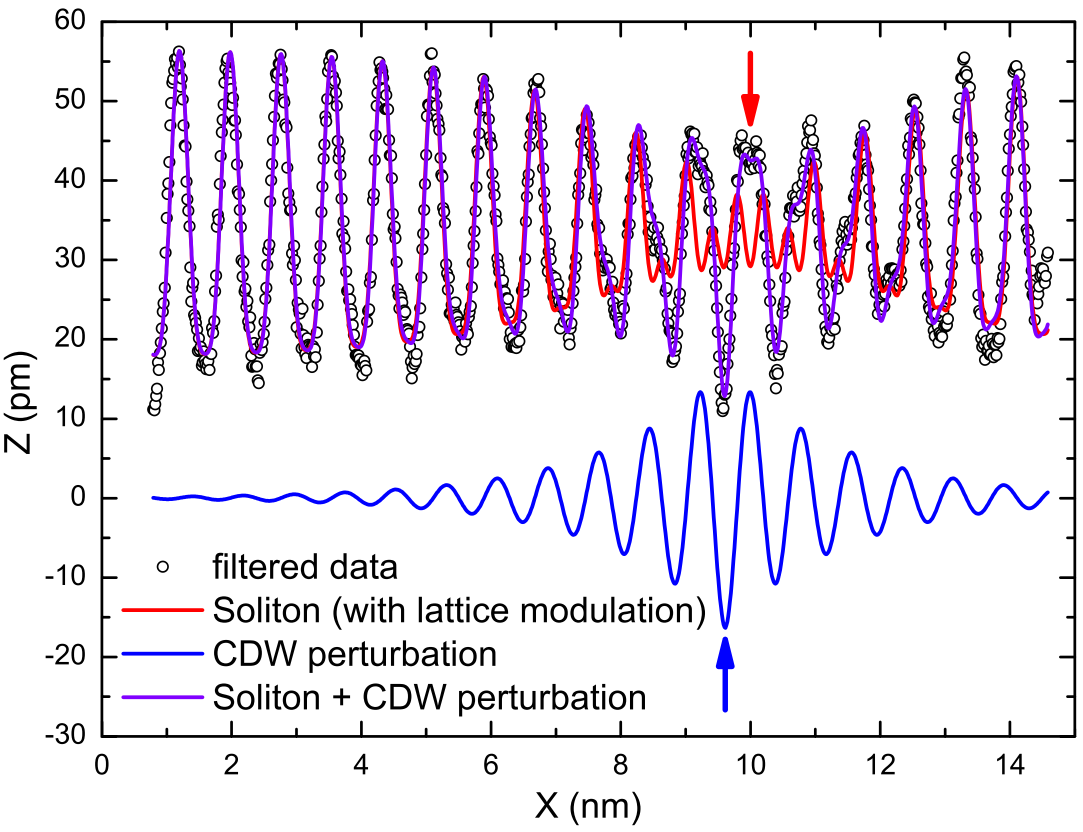


FIG. S3. STM line profiles (indicated by circles) of a long phase flip defect (PFD) along an upper In chain [Fig. 1(d)] as well as its fits. The chain shows a clear CDW phase shift similar to the long phase slip defect (PSD) [Fig. S2]. However, the data are deviated significantly from a soliton profile (red line) near the center (red arrow) of the long PFD, which is adjacent to the short defect of the neighboring wire. To describe this deviation, we consider a CDW perturbation induced by the neighboring defect. This perturbation could be dominated by the Friedel oscillations within the CDW coherence length [3]. Thus, we added a simple decaying amplitude oscillating at $2k_F(=\pi/a_0)$ as $Z_{pert.}(x) = A_0 \exp(-\frac{|x-x_0|}{\xi_0}) \cos\{\frac{\pi(x-x_0)}{a_0}\}$, where $x_0$ is the center of the CDW perturbation and $\xi_0$ is the decay length [4]. The blue solid line indicates the best fit of the perturbation ($\xi_0 = 1.82 \pm 0.07$ nm) and a resulting (violet) curve shows an almost perfect fit to the STM data. This suggests that the trapped soliton is coupled with an electron response to the trapping defect. Note that the center of the perturbation (blue arrow) is different from that of the soliton (red arrow) by $\sim 1a_0$, resulting in a $\pm\pi/2$ phase shift of the CDW perturbation with respect to the soliton. This is consistent with the fact that the neighboring short PFD, the trapping defect, is offset from the soliton center by $\frac{1}{2}a_0$ [Fig. 1(d)].

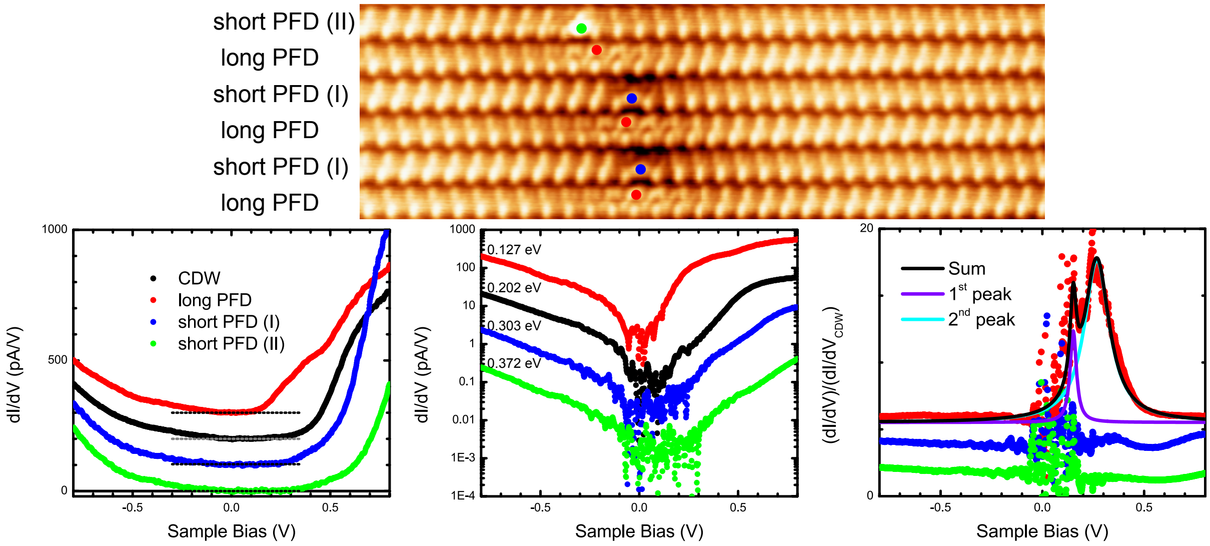


FIG. S4. Scanning tunneling spectroscopy (STS) spectra obtained at different phase defects. Colored dots in the above STM image indicate the centers of defects where we obtained the spectra. The data were taken using the lock-in detection of tunneling currents by adding a voltage modulation of 10–20 $\mathrm{mV_{rms}}$ at 500 Hz to the sample bias. Note that all spectra are offset for clarity. In order to determine gap widths more quantitatively from the spectra, we plotted each spectrum in logarithmic scale (bottom middle panel). In these semi-log plots, we could easily identify the gap region, where the very small noise conductance is observed due to the absence of density of states. On the normal CDW states away from defects (black dots), we could get a reliable gap width of 0.202 eV, consistent with the values reported previously (0.16 or 0.2 by STS [1, 5]; 0.25 by local transport [6]; and 0.34 eV by ARPES [7]), smaller and wider gaps for long and short phase defects, respectively. To empathize a difference from a normal CDW state, we normalized each spectrum with respect to that of the normal CDW state (bottom right panel). We observed two distinct peaks at the long PFDs (+0.152 and +0.268 eV) in contrast to other short PFDs. The lower peak (+0.152 eV) is a midgap state close to the upper gap edge (+0.156 eV) of the normal CDW state. We visualized a spatial distribution of this localized midgap state by obtaining the differential conductance map at +0.15 eV as shown in Fig. 1(e). For a soliton, a midgap state is expected to exist at $E_F$ [8] unlike the long PFDs. This discrepancy may be explained by a strong interaction of a commensurate CDW system with the underlying lattice, which lacks in an incommensurate CDW system [8]. The origin of the higher energy state at +0.268 eV is not clear at present. Further study is needed to gain a better understanding of the midgap state of the trapped soliton in a commensurtate CDW system.
